# Supplementary material for: Theory of triangular lattice quasi-one-dimensional charge-transfer solids
Source: arXiv:1904.03067 ancillary file (2019-08-20)
Supplement: Supplementary file 1 [file supplemental.pdf]

## Supplemental Material for "Theory of triangular lattice quasi-one-dimensional charge-transfer solids"

R. Torsten Clay,[1] Niladri Gomes,[2] and S. Mazumdar[2]

[1]*Department of Physics and Astronomy and HPC[2] Center for Computational Sciences, Mississippi State, MS 39762*
[2]*Department of Physics, University of Arizona, Tucson, AZ 85721*

(Dated: August 15, 2019)

### S.1. LATTICES

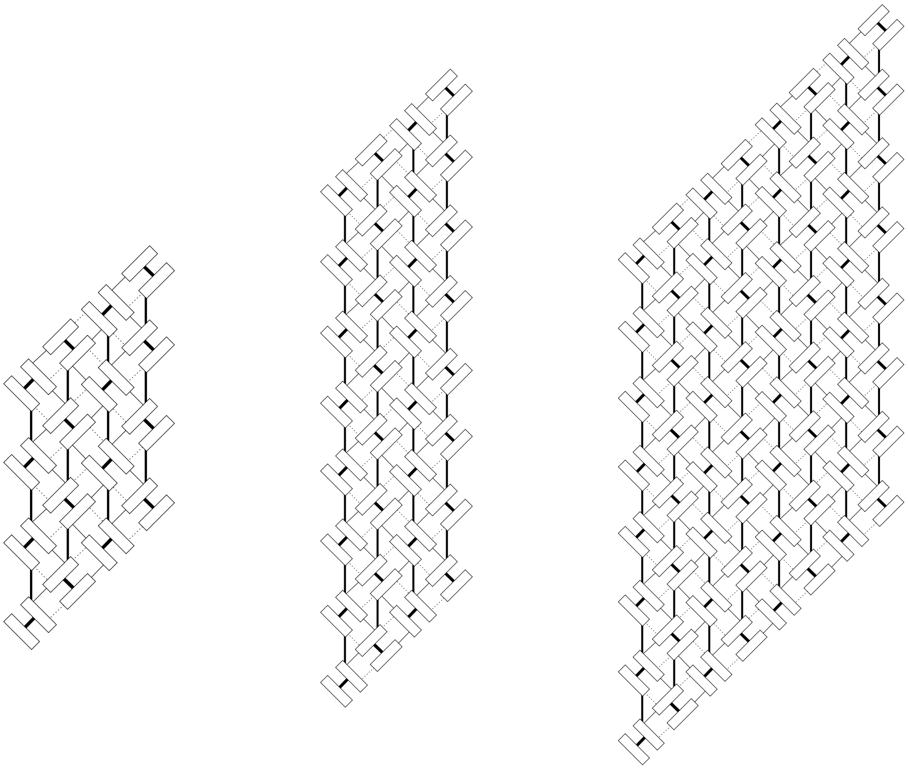

FIG. S1: 32, 64, and 128 site $\kappa$-(ET)$_2$X lattices considered in this paper. Periodic boundary conditions in all directions are assumed in each case. These are equivalent to 4×4, 8×4, and 8×8 lattices in terms of dimers, respectively.

### S.2. COMPUTATIONAL METHODS

*PIRG.* The Path Integral Renormalization Group (PIRG) method was used to calculate zero-temperature expectation values for the 32 site lattice, and to provide accurate trial wavefunctions for the 64 and 128 site lattices within CPMC (see below). PIRG was used because conventional Monte Carlo methods are limited by the fermion sign problem to either small Hubbard $U$ and/or high temperatures for frustrated lattices. The PIRG method is described in Reference [S1]. Within PIRG, the wavefunction is expanded as a sum over $L$ Slater determinants, and the projector operator $\exp(-\tau H)$ is used to project out the ground state from a random starting determinant [S1]. The method is exact at $U = 0$ and for each $L$ PIRG calculations are variational. For the 32 site data we first minimized the variational energy for $L = 1$, followed by optimizing the variational state at $L = 8$. We then continued calculations to larger $L$, doubling ($L$ =16, 32, ...) $L$ at each step. We used maximum $L$'s of up to 768. The finite basis bias is then removed by extrapolating quantities as a function of the energy variance ΔE [S1]. For the results presented here, we typically used a linear extrapolation in ΔE for the three largest $L$ used, i.e. $L$={256, 512, 768}. The error bars we report for PIRG results are the statistcal uncertainty in the extrapolated values.

Several additional techniques are essential to improve the accuracy of the PIRG. First, we incorporated lattice and spin symmetries using projection operators of the QP-PIRG method of Reference [S2]. The use of lattice and spin symmetries has

been shown to drastically reduce the $L$ required to obtain accurate results with PIRG [S2]. Here we used the more accurate method of incorporating symmetries during projection (QP-PIRG) as opposed to afterwards (PIRG-QP) [S2]. For the lattice symmetry we used the full space group of the lattice (translations and point symmetries). For spin, we projected using the spin parity operator, which separates even and odd values of total spin $S$. All results here are for the even spin parity subspace. Second, it has been observed that in certain cases the PIRG method can be trapped in excited states [S3]. To help prevent this, in addition to the PIRG projection operator, we used a random simulated annealing-like modification of the Slater determinants [S3][S4]. Furthermore, several starting states were chosen for the projection, and their final energy compared.

PIRG has been extensively benchmarked against other methods. We previously compared the pair-pair correlations from PIRG and exact diagonalization on a 4×4 frustrated lattice and found essentially perfect agreement [S4,5]. For larger lattices, PIRG has further been checked against conventional quantum Monte Carlo for systems where there is no sign problem, such as the half-filled square lattice Hubbard model [S2].

*CPMC.* Constrained Path Monte Carl (CPMC) is a ground-state projector QMC method [S6]. Like PIRG, CPMC works in the space of Slater determinants. This space is overcomplete, which results in contributions to the ground state wavefunction that are both positive and negative. The Monte Carlo sampling is confined to the region where the overlap between each random walker $|\phi\rangle$ and a trial wavefunction $|\Psi_T\rangle$ is positive [S6]. This eliminates the loss of precision known as the fermion sign problem, but introduces an approximation into the method. The results presented here for $S(\mathbf{Q})$ and the pairing correlations for 64 and 128 sites used the PIRG $L=1$ wavefunction for $|\Psi_T\rangle$. As with PIRG space group and spin parity symmetries were used in the calculation. We used an imaginary time discretization of $\Delta\tau = 0.1$ with a second-order Trotter approximation; the additional systematic error due to this approximation is negligible. The charge order parameter in Fig. 4(b) is less sensitive to the effect of correlations than long-range correlations like $P(r)$; for the results of Fig. 4(b) the CPMC method with a free-electron trial function was used.

## S.3. PAIRING CORRELATIONS

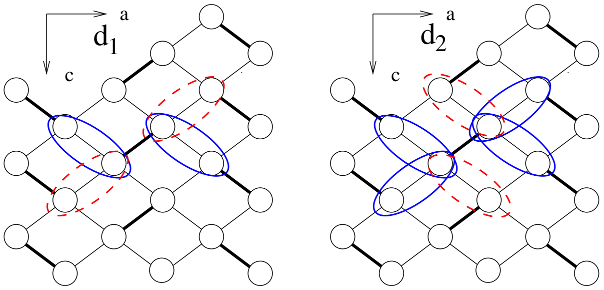


FIG. S2: Pairing symmetries considered in our calculations. Blue, solid (red, dashed) ellipses indicate nearest-neighbor singlet pairs with opposite signs in $\Delta^\dagger$. The $d_1$ symmetry is similar to $d_{x^2-y^2}$ pairing with four nodes nodes along the crystal axes. The $d_2$ symmetry also has four nodes, but with mixed $s+d_{x^2-y^2}$ character.

We calculate equal-time pair-pair correlations, defined as $P_{ij} = \langle \Delta_i^\dagger \Delta_j \rangle$ with

$$\Delta_i^\dagger = \mathcal{N} \sum_\nu \frac{1}{\sqrt{2}} (c^\dagger_{i_{\nu,1},\uparrow} c^\dagger_{i_{\nu,2},\downarrow} - c^\dagger_{i_{\nu,1},\downarrow} c^\dagger_{i_{\nu,2},\uparrow}). \quad (1)$$

In Eq. 1 the index $i$ refers to a *dimer* in the lattice. The index $\nu$ runs over either 4 or 6 pairs centered on dimer $i$ as shown in Fig. S2. The indices $i_{\nu,1}$ and $i_{\nu,2}$ refer to the molecular sites composing this dimer; $\mathcal{N}$ is an overall normalization factor. We define $\bar{P}$ as the average the long-range $P(r) \equiv P(|r_{ij}|)$ for $r > 2$, where $r$ is defined in units of the dimer-dimer distance on a square lattice as in Fig. 1(b):

$$\bar{P} = \frac{1}{N_P} \sum_{|r_{ij}|>2} P(r). \quad (2)$$

To measure the enhancement of pairing by $U$ we divide $\bar{P}(U)$ by its uncorrelated ($U=0$) value. We define the enhancement factor $\Theta_P = \bar{P}(U)/\bar{P}(U=0) - 1$. For certain densities a quantum phase transition occurs at a small $U_c \lesssim 0.1$ eV due to the breaking of single-particle degeneracies. In these cases the pair-pair correlations typically change discontinuously at $U_c$, and

we instead define $\Theta_P = \bar{P}(U)/\bar{P}(U_0) - 1$, with $U_0 > U_c$. In the plots that follow, filled symbols indicate the $\bar{P}(U_0)$ chosen to normalize $P(\bar{U})$.

In two lattices (32 sites $CF_3SO_3$ layer B, and 32 sites $B(CN)_4$) see Figs. S5–S8) a quantum phase transition occurs at $U = U_c$ ($U_c \approx 0.4$ eV for $CF_3SO_3$ layer B and $U_c \approx 0.15$ eV for $B(CN)_4$) to an insulating state with strong **Q**=$(\pi, \pi)$ AFM order. For $U < U_c$ pairing correlations are enhanced. We find no evidence that such a transition persists for larger lattices and conclude it is a finite-size effect. Except for this lattice, we find only enhancement of $d_2$ pairing by $U$; in all other cases $d_1$ pairing is suppressed by $U$.

**S.3.1. 32 sites, $\kappa$-$CF_3SO_3$ layer A**

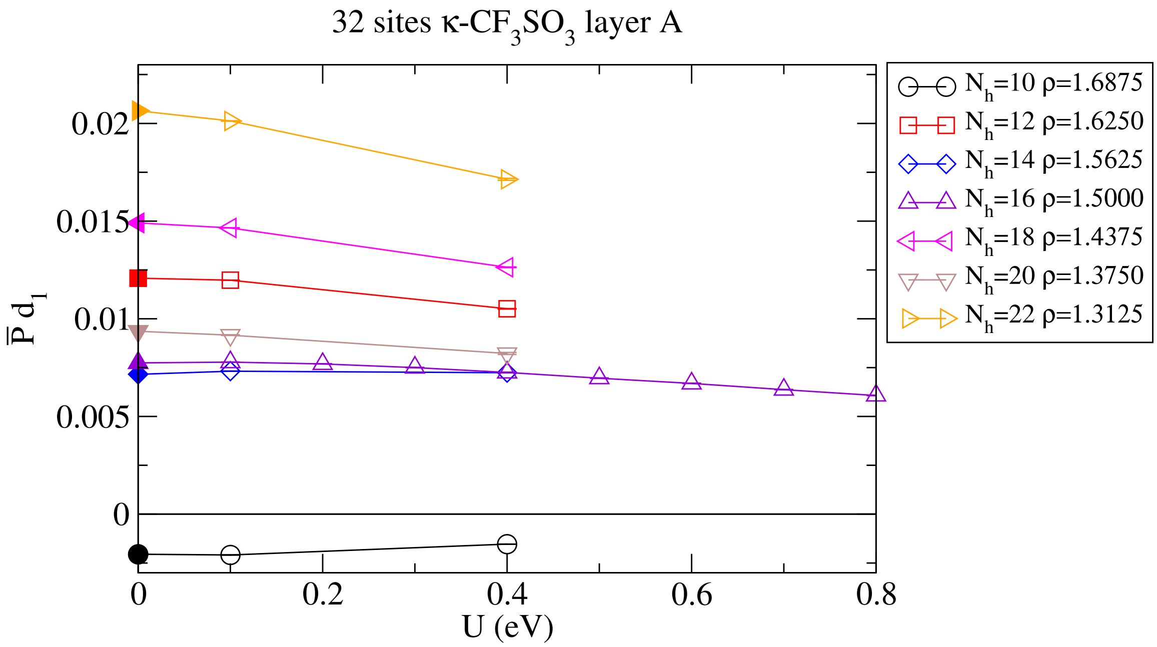


FIG. S3: $\bar{P}$ for $d_2$ ($d_{x^2-y^2}$) pairing versus $U$ for the 32 site $\kappa$-$CF_3SO_3$ layer A lattice. All calculations used the PIRG method. There is no enhancement of $d_1$ pairing at any density.

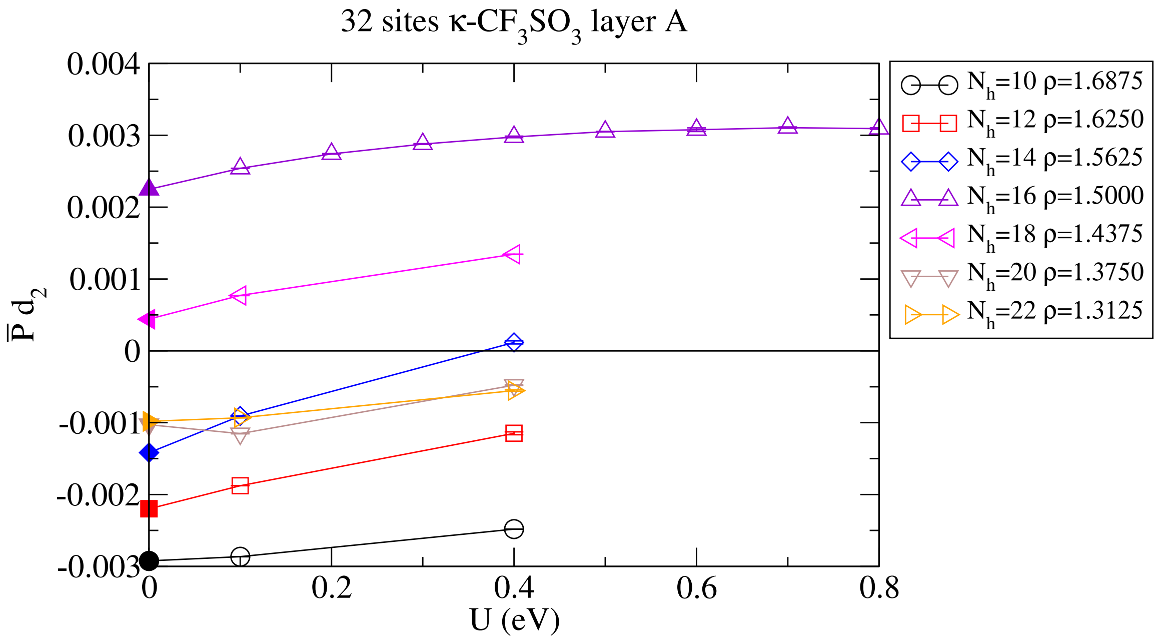


FIG. S4: $\bar{P}$ for $d_2$ ($s + d_{x^2-y^2}$) pairing versus $U$ for the 32 site $\kappa$-$CF_3SO_3$ layer A lattice. All calculations used the PIRG method. $d_2$ pairing is enhanced at $\rho = 1.5000$ and $\rho = 1.4375$ (see Fig. 5(a)). $\bar{P}$ for other densities is negative and decreasing in magnitude.

### S.3.2. 32 sites, $\kappa$-$CF_3SO_3$ layer B

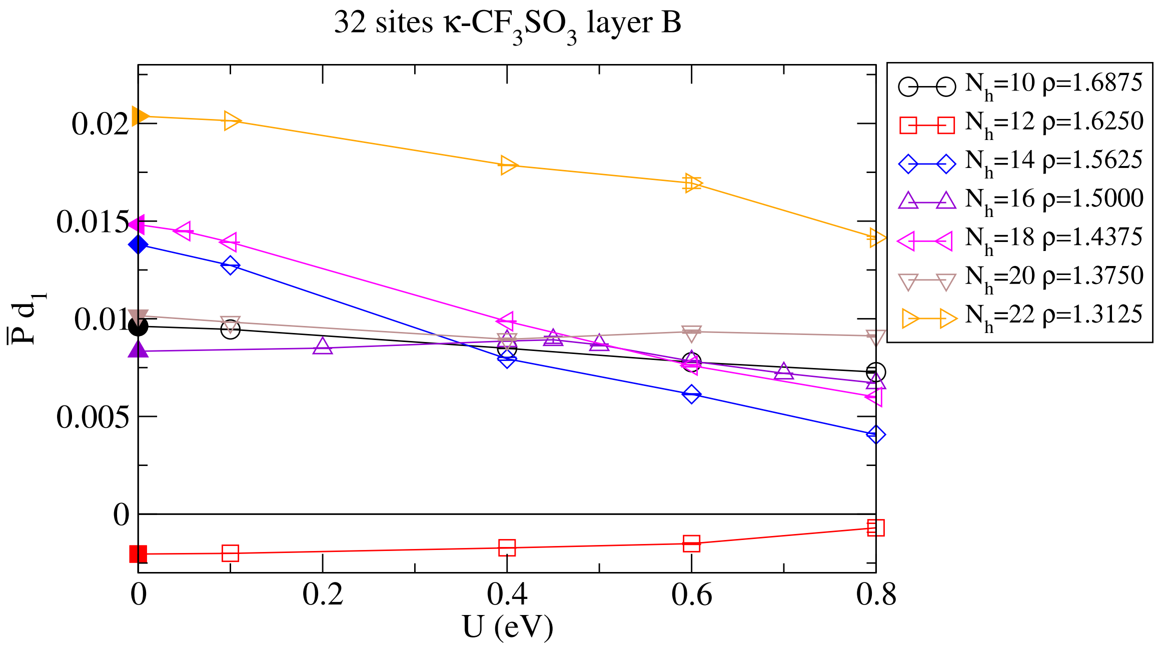


FIG. S5: $\bar{P}$ for $d_1$ ($d_{x^2-y^2}$) pairing versus $U$ for the 32 site $\kappa$-$CF_3SO_3$ layer B lattice. All calculations used the PIRG method. There is no enhancement of $d_1$ pairing at any density.

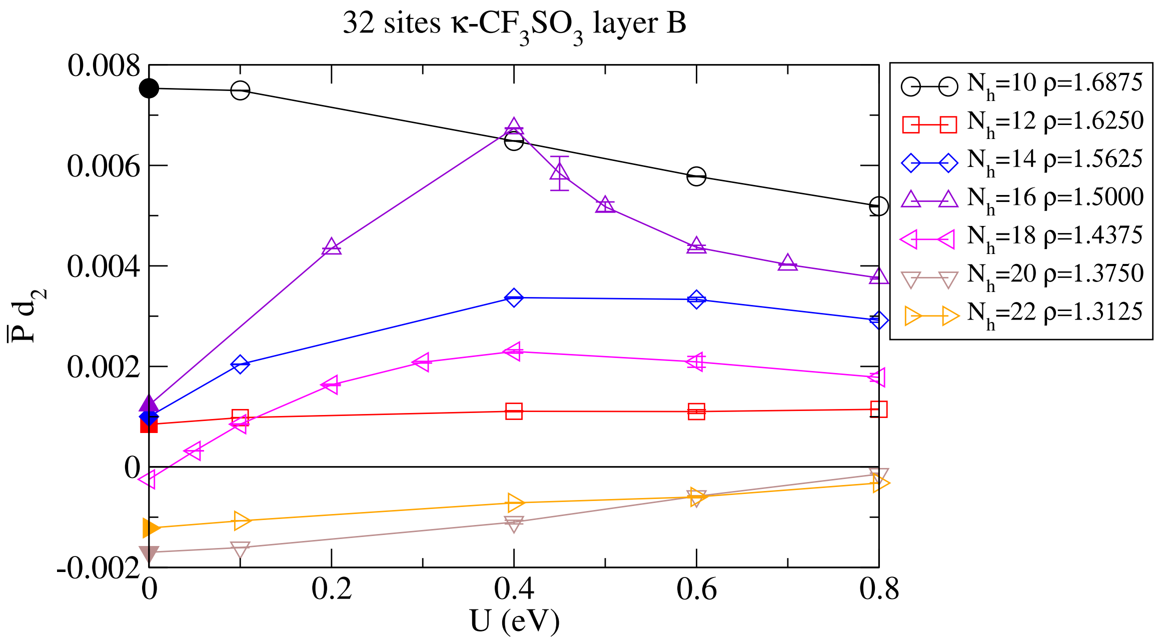


FIG. S6: $\bar{P}$ for $d_2$ ($s + d_{x^2-y^2}$) pairing versus $U$ for the 32 site $\kappa$-$CF_3SO_3$ layer B lattice. All calculations used the PIRG method. $d_2$ pairing is strongly enhanced at $\rho = 1.5000$ (see Fig. 5(b)). Pairing is also enhanced at $\rho = 1.4375$ and $\rho = 1.5625$. $\rho = 1.4375$ is not plotted (see "$\star$" in Fig. 5(b)) because the $U = 0$ value is close to zero here. At other densities the magnitude of $\bar{P}$ decreases with $U$. For $\rho = 1.5000$ a transition to an insulating AFM state occurs at $U \sim 0.4$ eV (see main text).

### S.3.3. 32 sites, B(CN)$_4$

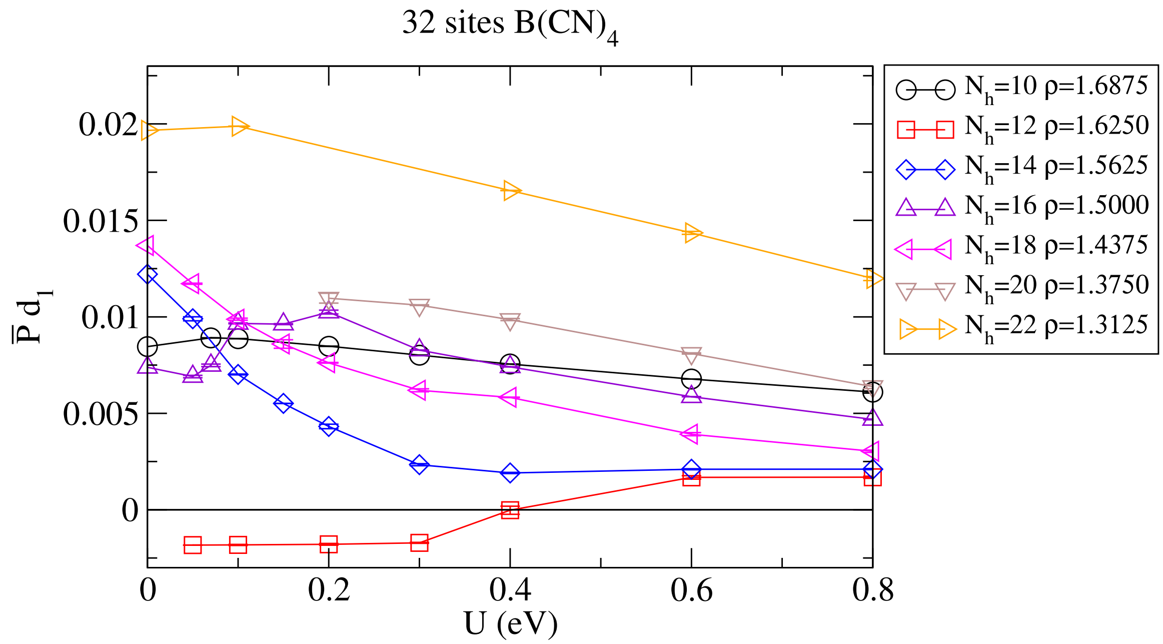


FIG. S7: $\bar{P}$ for $d_1$ ($d_{x^2-y^2}$) pairing versus $U$ for the 32 site B(CN)$_4$ lattice. All calculations used the PIRG method. $d_1$ pairing is enhanced at $\rho = 1.5000$. There is no enhancement at other densities.

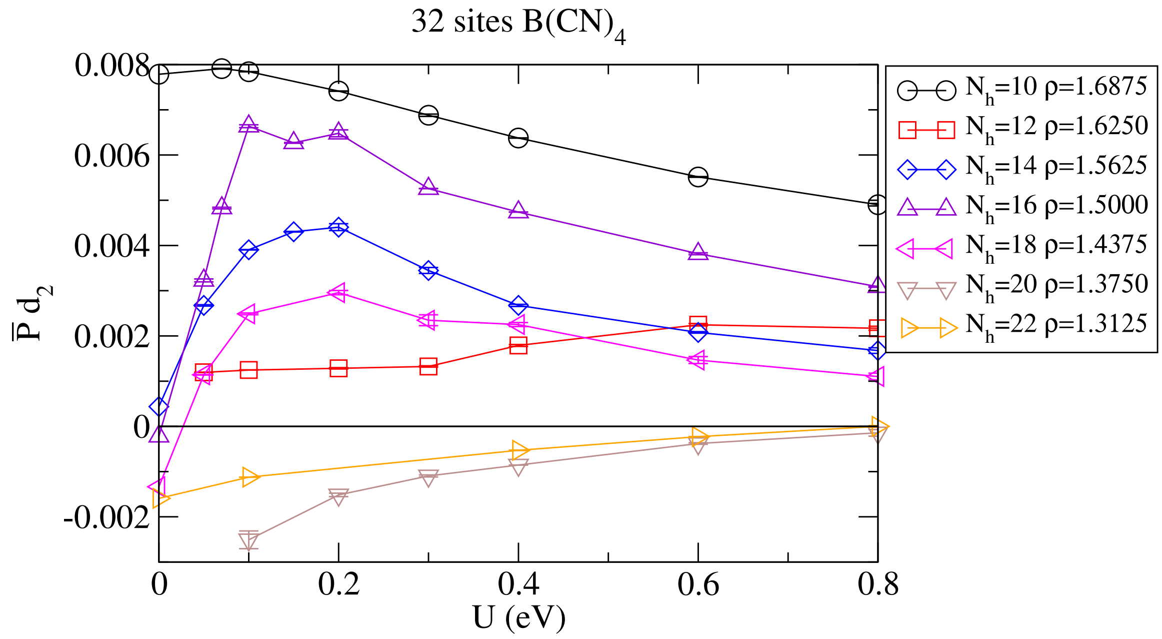


FIG. S8: $\bar{P}$ for $d_2$ ($s + d_{x^2-y^2}$) pairing versus $U$ for the 32 site B(CN)$_4$ lattice. All calculations used the PIRG method. $d_2$ pairing is enhanced for $\rho = 1.4365$, $\rho = 1.5000$, and $\rho = 1.5625$. There is no enhancement at other densities. For $\rho = 1.5000$ a transition to an insulating AFM state takes place at $U \approx 0.15$ eV (see main text).

### S.3.4. 64 sites, κ-$CF_3SO_3$ layer A

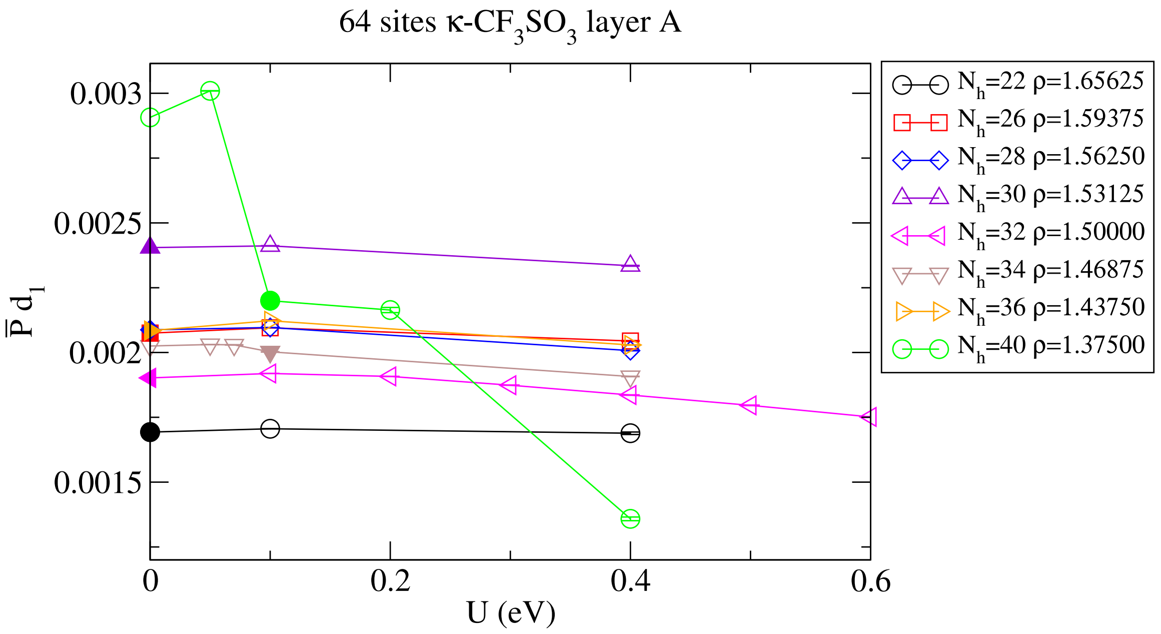


FIG. S9: $\bar{P}$ for $d_1$ ($d_{x^2-y^2}$) pairing versus $U$ for the 64 site κ-$CF_3SO_3$ layer A lattice. All calculations used CPMC with PIRG trial wavefunctions. A level-crossing transition occurs for $\rho = 1.375$ at $U \approx 0.15$ eV; we ignore smaller $U$ values here. There is no enhancement of $d_1$ pairing at any density.

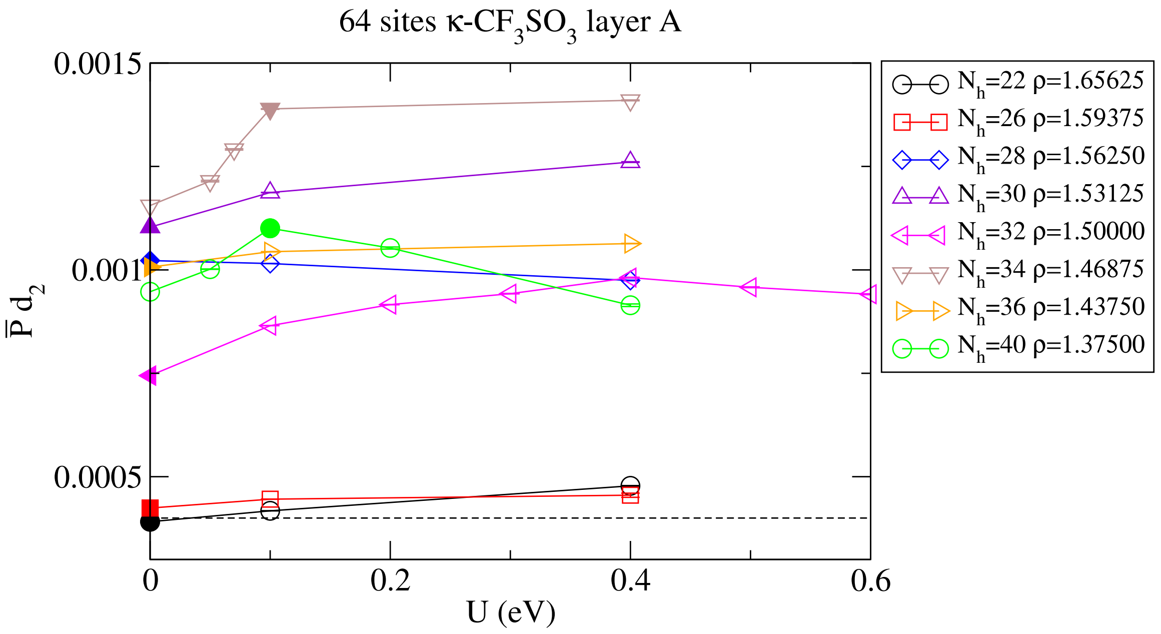


FIG. S10: $\bar{P}$ for $d_2$ ($s + d_{x^2-y^2}$) pairing versus $U$ for the 64 site κ-$CF_3SO_3$ layer A lattice. All calculations used CPMC with PIRG trial wavefunctions. A level-crossing transition occurs for $\rho = 1.375$ at $U \approx 0.15$ eV; we ignore smaller $U$ values here. Densities $\rho = 1.5000$ and $\rho = 1.53125$ are significantly enhanced (see Fig. 5(c)). $\bar{P}$ at other densities decreases with $U$ or is only weakly enhanced. $\rho = 1.65625$ was removed from Fig. 5(c) because $\bar{P}(U = 0)$ is very small (see "⋆" in Fig. 5(c)). $\bar{P}$

**S.3.5. 64 sites, κ-$CF_3SO_3$ layer B**

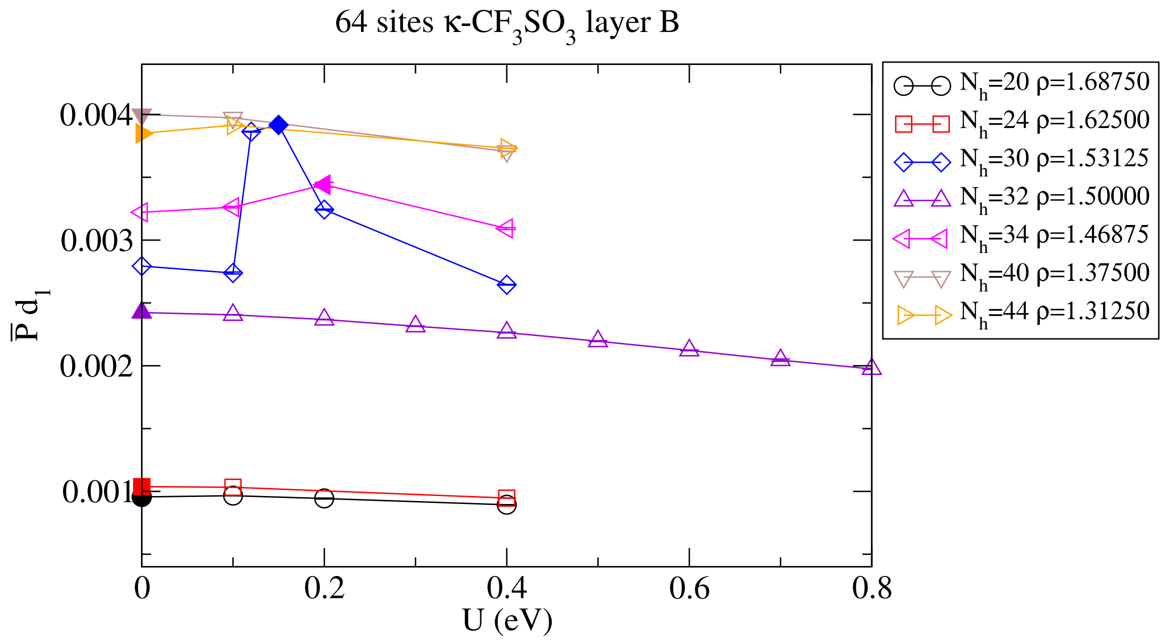


FIG. S11: $\bar{P}$ for $d_1$ ($d_{x^2-y^2}$) pairing versus $U$ for the 64 site κ-$CF_3SO_3$ layer B lattice. All calculations used CPMC with PIRG trial wavefunctions. A level-crossing transition occurs for $\rho = 1.53125$ at $U \approx 0.15$ eV; we ignore smaller $U$ values here. There is no enhancement of $d_1$ pairing at any density.

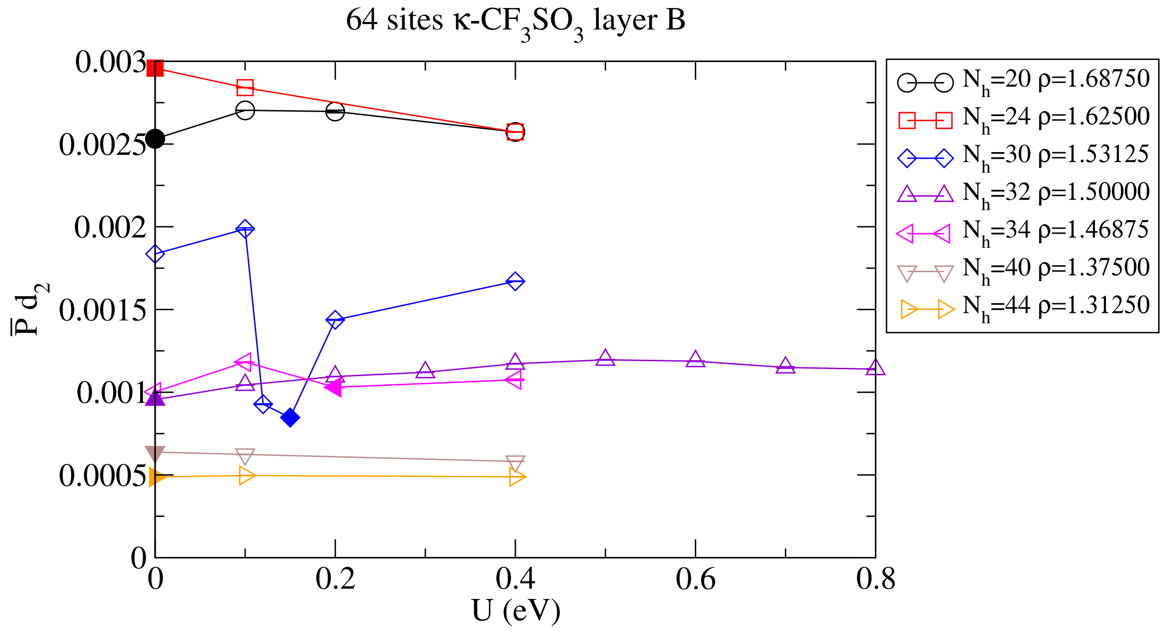


FIG. S12: $\bar{P}$ for $d_2$ ($s + d_{x^2-y^2}$) pairing versus $U$ for the 64 site κ-$CF_3SO_3$ layer B lattice. All calculations used CPMC with PIRG trial wavefunctions. A level-crossing transition occurs for $\rho = 1.53125$ at $U \approx 0.15$ eV; we ignore smaller $U$ values here. $\bar{P}$ for $\rho = 1.50000$ and $\rho = 1.53125$ is enhanced (see Fig. 5(d)). There is no enhancement at other densities.

### S.3.6. 128 sites, $\kappa$-$CF_3SO_3$ layer A

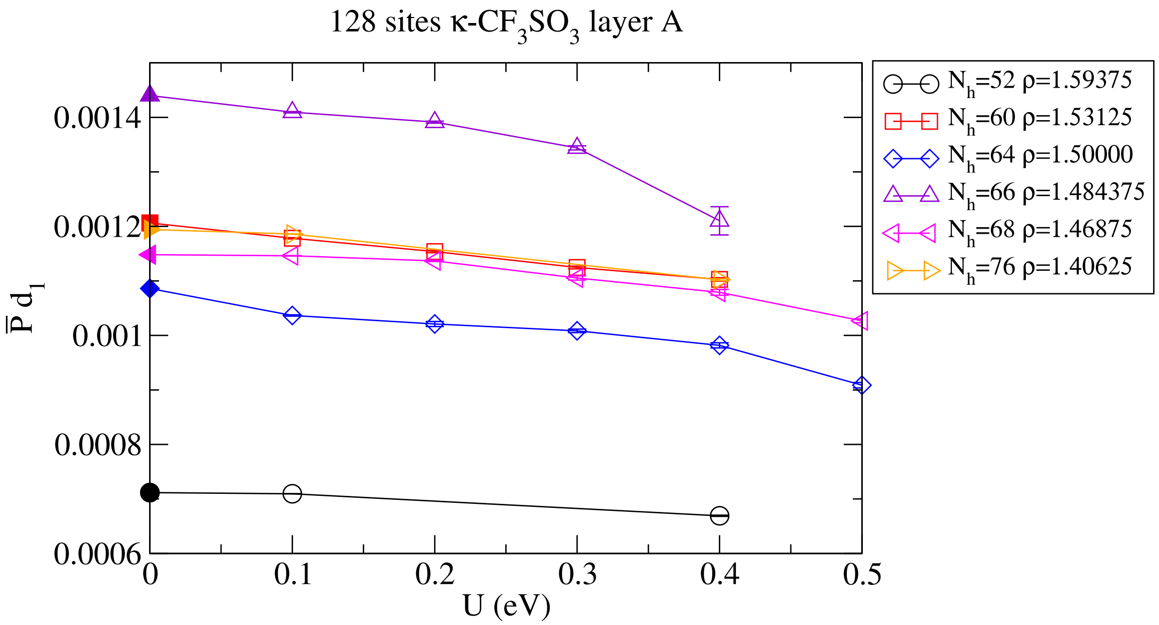


FIG. S13: $\bar{P}$ for $d_1$ ($d_{x^2-y^2}$) pairing versus $U$ for the 128 site $\kappa$-$CF_3SO_3$ layer A lattice. All calculations used CPMC with PIRG trial wavefunctions. There is no enhancement of $d_1$ pairing at any density.

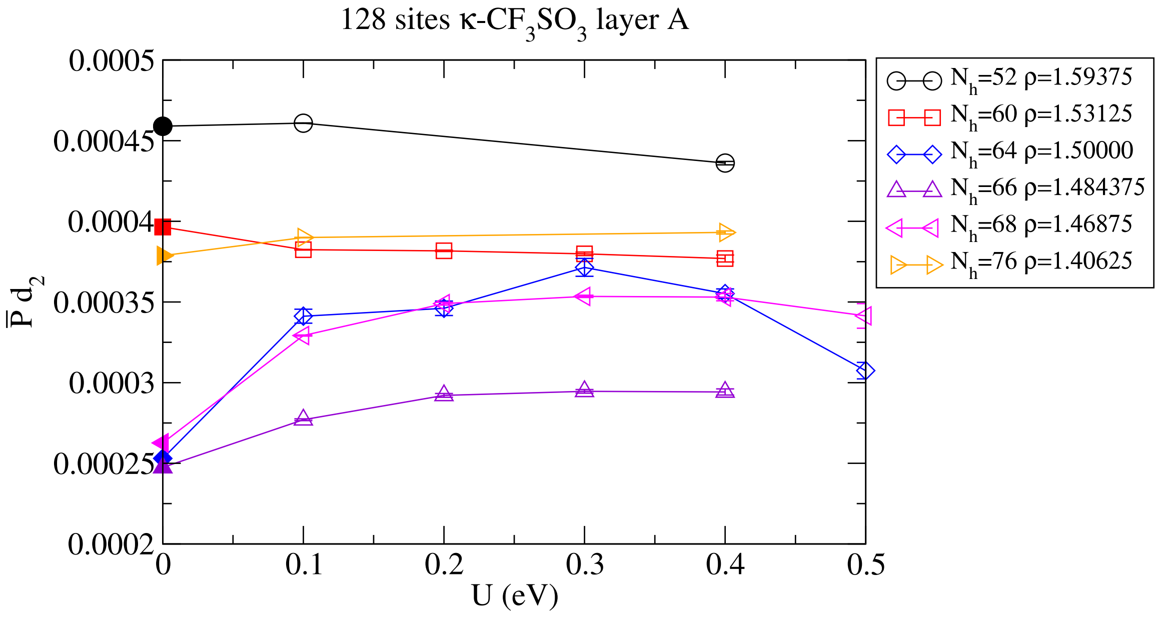


FIG. S14: $\bar{P}$ for $d_2$ ($s + d_{x^2-y^2}$) pairing versus $U$ for the 128 site $\kappa$-$CF_3SO_3$ layer A lattice. All calculations used CPMC with PIRG trial wavefunctions. $d_2$ pairing at $\rho = 1.5$ and neighboring densities are enhanced (see Fig. 5(e)).

### S.3.7. 128 sites, $\kappa$-$CF_3SO_3$ layer B

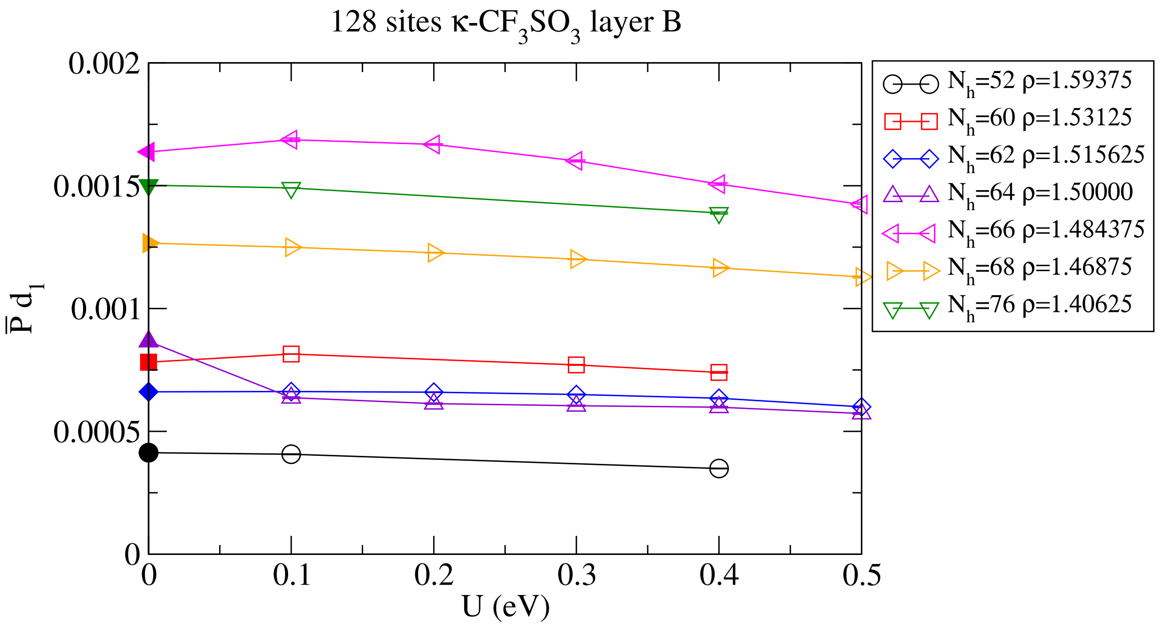


FIG. S15: $\bar{P}$ for $d_1$ ($d_{x^2-y^2}$) pairing versus $U$ for the 128 site $\kappa$-$CF_3SO_3$ layer B lattice. All calculations used CPMC with PIRG trial wavefunctions. There is no enhancement of $d_1$ pairing at any density.

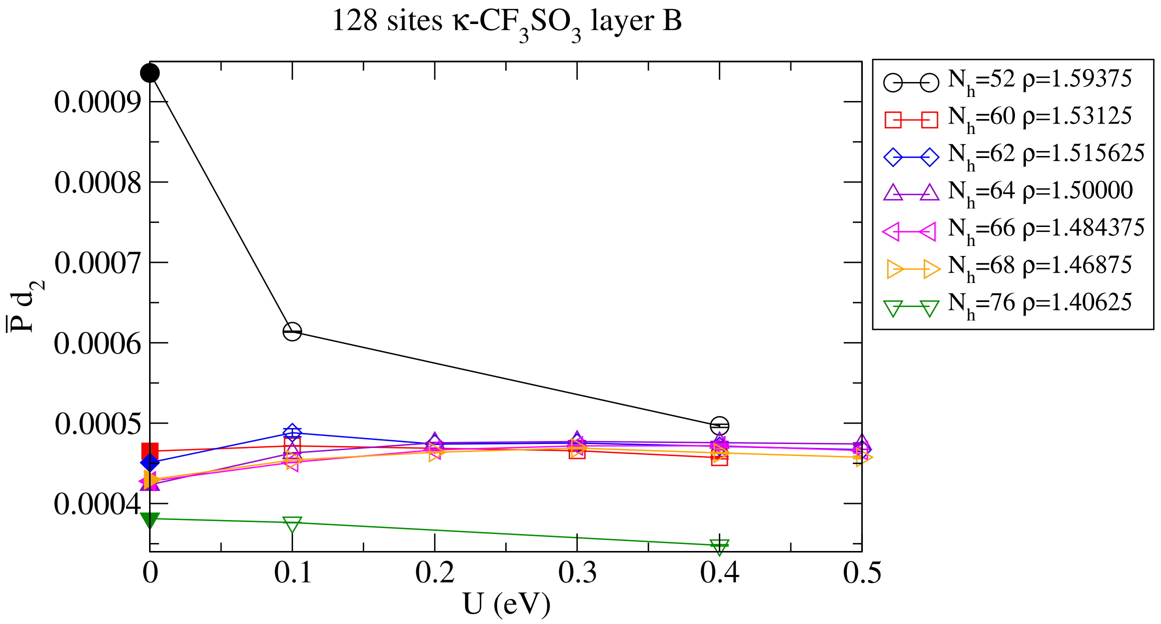


FIG. S16: $\bar{P}$ for $d_2$ ($s + d_{x^2-y^2}$) pairing versus $U$ for the 128 site $\kappa$-$CF_3SO_3$ layer B lattice. All calculations used CPMC with PIRG trial wavefunctions. $d_2$ pairing is enhanced for $\rho = 1.5000$, $\rho = 1.484375$, and $\rho = 1.46875$, and slightly at $\rho = 1.515625$. There is no enhancement for the densities far away from $\rho = 1.5000$.

## S.4. CHARGE ORDER PATTERN IN THE PAIRED ELECTRON CRYSTAL

In the PEC state, charge order (CO) is stabilized by the cooperative effects of nearest-neighbor singlet formation and electron-phonon interactions rather than nearest-neighbor Coulomb interactions $V_{ij}$ which stabilizes Wigner crystal CO [S7][S8]. In order to stabilize singlet formation in a 2D lattice the CO associated with a PEC state must therefore have a specific pattern, ...0110... in two of the dominant lattice directions in a frustrated lattice, and ...1010... in the third direction [S7][S8]. When following the dominant directions one must follow *along the path of the strongest inter-molecular bonds* $t_{b1}$, $t_{b2}$, *and* $t_p$ [S7][S8]. We take the effective $t_x$, $t_y$, and $t'$ directions (see Fig. 1) as the dominant lattice directions and follow only the strongest bonds of the lattice, ignoring the weaker $t_q$ bonds. There are then three possible PEC states:

(a) ...1100... along $t_y$ and $t'$ and ...1010... along $t_x$ (see Fig. S17(a))

(b) ...1100... along $t_x$ and $t_y$ and ...1010... along $t'$ (see Fig. S17(b))

(c) ...1100... along $t_x$ and $t'$ and ...1010... along $t_y$ (equivalent by symmetry to (a))

Fig. S17 shows the possible PEC CO patterns: Although two PEC states are possible, that of Fig. S17(a) is the most likely

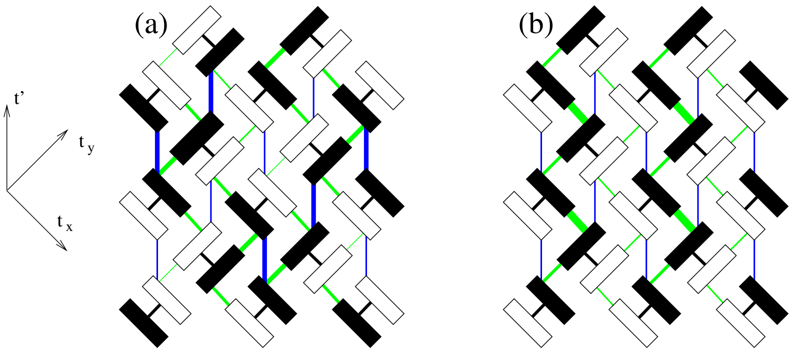


FIG. S17: Possible PEC CO patterns in the $\kappa$-(ET)$_2$X lattice. $t_p$ ($t_{b2}$) bonds are shown in green (blue). Thicker lines correspond to stronger bond orders. (a) ...0110... CO along the $t'$ and $t_y$ effective directions and ...1010... CO along the $t_x$ effective direction. This is the same CO pattern shown in Fig. 4. A similar PEC state exists with the roles of $t_x$ and $t_y$ interchanged. (b) ...0110... CO along the $t_x$ and $t_y$ effective directions and ...1010... CO along the $t'$ effective direction.

candidate to explain the spin gap state in $\kappa$-(ET)$_2$B(CN)$_4$, because the pattern of Fig. S17(a) has alternation of the $t_{b2}$ bonds, which are the strongest interdimer bonds. In contrast the pattern of Fig. S17(b) has alternating $t_p$ bonds which are much weaker. In such a case the spin gap would likely be very small We note that the pattern of Fig. S17(a) doubles the periodicity of the lattice along both crystal directions.


[S1] T. Kashima and M. Imada. Path-integral renormalization group method for numerical study on ground states of strongly correlated electronic systems. *J. Phys. Soc. Jpn.*, 70:2287–2299, 2001.

[S2] T. Mizusaki and M. Imada. Quantum-number projection in the path-integral renormalization group method. *Phys. Rev. B*, 69:125110, 2004.

[S3] T. Yoshioka, A. Koga, and N. Kawakami. Mott transition in the Hubbard model on checkerboard lattice. *J. Phys. Soc. Jpn.*, 77:104702, 2008.

[S4] S. Dayal, R. T. Clay, and S. Mazumdar. Absence of long-range superconducting correlations in the frustrated $\frac{1}{2}$-filled band Hubbard model. *Phys. Rev. B*, 85:165141, 2012.

[S5] N. Gomes, W. Wasanthi De Silva, T. Dutta, R. T. Clay, and S. Mazumdar. Coulomb enhanced superconducting pair correlations in the frustrated quarter-filled band. *Phys. Rev. B*, 93:165110, 2016.

[S6] S. Zhang, J. Carlson, and J. E. Gubernatis. Constrained path Monte Carlo method for fermion ground states. *Phys. Rev. B*, 55:7464–7477, 1997.

[S7] H. Li, R. T. Clay, and S.Mazumdar. The paired-electron crystal in the two-dimensional frustrated quarter-filled band. *J. Phys.: Condens. Matter*, 22:272201, 2010.

[S8] S. Dayal, R. T. Clay, H. Li, and S. Mazumdar. Paired electron crystal: Order from frustration in the quarter-filled band. *Phys. Rev. B*, 83:245106, 2011.
